# Supplementary material for: Cu$_2$ZnSiTe$_4$: A potential thermoelectric material with promising electronic transport
Source: arXiv:2401.05903 ancillary file (2024-01-12)
Supplement: Supplementary file 1 [file suppl.pdf]

# Cu<sub>2</sub>ZnSiTe<sub>4</sub> as a potential thermoelectric material with promising electronic transport

Himanshu Sharma<sup>1</sup>, Bhawna Sahni<sup>1</sup>, Tanusri Saha-Dasgupta<sup>2</sup> and Aftab Alam<sup>1</sup>

aftab@iitb.ac.in

<sup>1</sup>*Department of Physics, Indian Institute of Technology, Bombay, Powai, Mumbai 400 076, India*

<sup>2</sup>*Department of Condensed Matter Physics and Material Sciences, S. N. Bose National Centre for Basic Sciences, JD Block, Sector III, Salt Lake, Kolkata, West Bengal 700106, India*

## SUPPLEMENTARY INFORMATION

Here we provide, additional information regarding band structure and effect of spin-orbit coupling on it. Later we have shown the carrier relaxation time and its variation with respect to temperature.

### I. BAND STRUCTURE

The effect of spin-orbit coupling (SOC) can be seen from Fig. SI (a) and (b). The major effect is the reduction of band gap from 0.74 eV to 0.58 eV after including SOC. The splitting can be seen at high symmetry point  $\Gamma$  and as well as in other high symmetry directions. The effect of SOC can be seen more on the valence bands at high symmetry point  $\Gamma$  as compared to the conduction band. In Fig.SI (a) there are two bands coinciding at  $\Gamma$  in valence bands, which splits with a very small energy of 28 meV with the inclusion of SOC. Thus, SOC has a profound effect on the electronic structure of Cu<sub>2</sub>ZnSiTe<sub>4</sub>.

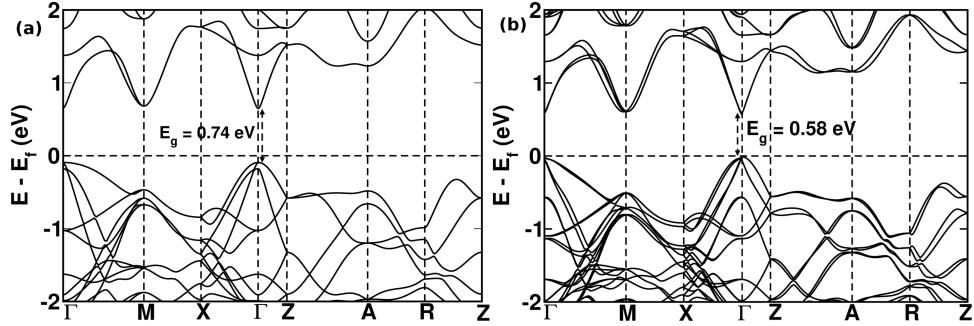

FIG. SI. Band structure of Cu<sub>2</sub>ZnSiTe<sub>4</sub> (a) without spin-orbit coupling, (b) with spin-orbit coupling effect

### II. RELAXATION TIME FORMALISM

Relaxation time for electron and hole transport in Cu<sub>2</sub>ZnSiTe<sub>4</sub> was estimated using a code, Ab-initio Scattering and Transport (AMSET)[1]. We have calculated the transport properties using four scattering mechanisms which are included in AMSET. They are acoustic deformation potential scattering, ionized impurity scattering, polar optical phonon scattering and piezoelectric scattering. The mode-dependent scattering rates are calculated using Born approximation. The differential scattering rate from initial state  $|nk\rangle$  to final state  $|mk+q\rangle$  using Fermi golden rule is calculated as:

$$\tau_{nk \rightarrow mk+q}^{-1} = \frac{2\pi}{\hbar} |g_{nm}(k, q)|^2 \delta(\epsilon_{nk} - \epsilon_{mk+q}), \quad (1)$$

where  $g_{nm}(k, q)$  is the matrix element for scattering from state  $|nk\rangle$  into state  $|mk+q\rangle$  and  $\epsilon_{nk}$  is the energy of the state  $|nk\rangle$ .

The band structure of the material is determined by the crystal potential which gets deformed by the lattice perturbation due to the thermal vibration of atom. The acoustic deformation potential is calculated considering the potential

perturbation has linear dependence upon relative volume change. A more general acoustic deformation potential matrix element is given by:

$$g_{nm}^{ad}(k, q) = \sqrt{k_B T} \sum_{G \neq -q} \left[ \frac{\tilde{D}_{nk} : \tilde{S}_l}{cl\sqrt{\rho}} + \frac{\tilde{D}_{nk} : \tilde{S}_{t_1}}{ct_1\sqrt{\rho}} + \frac{\tilde{D}_{nk} : \tilde{S}_{t_2}}{ct_2\sqrt{\rho}} \right] \langle mk + q | e^{i(q+G) \cdot r} | nk \rangle \quad (2)$$

where  $\hat{S} = \hat{q} \otimes \hat{u}$  is the unit strain for an acoustic mode,  $\tilde{D}_{nk} = D_{nk} + v_{nk} \otimes v_{nk}$  in which  $D_{nk}$  is the rank 2 deformation potential tensor,  $\hat{u}$  is the unit vector of phonon polarization, and the subscripts  $l$ ,  $t_1$  and  $t_2$  indicate properties belonging to the longitudinal and transverse modes.

In polar material, the dipole moment gets perturbed due to lattice vibrations. An electric field is created due to this perturbation which scatters the carriers. Since there are two possible modes of vibration, if vibrations are due to acoustic modes, it is called Piezoelectric scattering and if it is due to optical modes, it is known as Polar optical phonon scattering. A general expression for PIE scattering rate is given by:

$$g_{nm}^{pie}(k, q) = \sqrt{k_B T} \sum_{G \neq -q} \left[ \frac{\hat{n}h : \tilde{S}_l}{cl\sqrt{\rho}} + \frac{\hat{n}h : \tilde{S}_{t_1}}{ct_1\sqrt{\rho}} + \frac{\hat{n}h : \tilde{S}_{t_2}}{ct_2\sqrt{\rho}} \right] \frac{\langle mk + q | e^{i(q+G) \cdot r} | nk \rangle}{|q + G|} \quad (3)$$

where  $h$  is full piezoelectric stress tensor and  $\hat{n} = \frac{q+G}{|q+G|}$  is unit vector in the direction of scattering. Expression for POP scattering rate is given by:

$$g_{nm}^{po}(k, q) = \left[ \frac{\hbar\omega_{po}}{2} \right]^{1/2} \sum_{G \neq -q} \left( \frac{1}{\hat{n} \cdot \epsilon_{\infty} \cdot \hat{n}} - \frac{1}{\hat{n} \cdot \epsilon_s \cdot \hat{n}} \right)^{1/2} \frac{\langle mk + q | e^{i(q+G) \cdot r} | nk \rangle}{|q + G|} \quad (4)$$

where  $\epsilon_s$  and  $\epsilon_{\infty}$  are the static and high-frequency dielectric tensors and  $\omega_{po}$  is the polar optical phonon frequency. PIE is important at low temperature whereas POP dominates above room temperature.

Ionised impurity in semiconductors creates an electric field which can affect the trajectory of charge carriers. Due to this electric field, acceptor or donor impurities start to attract the opposite charge carriers around them. Accumulation of charge carriers in the vicinity of ionised impurity screens the effective potential. The matrix element for Ionised impurity scattering is given by:

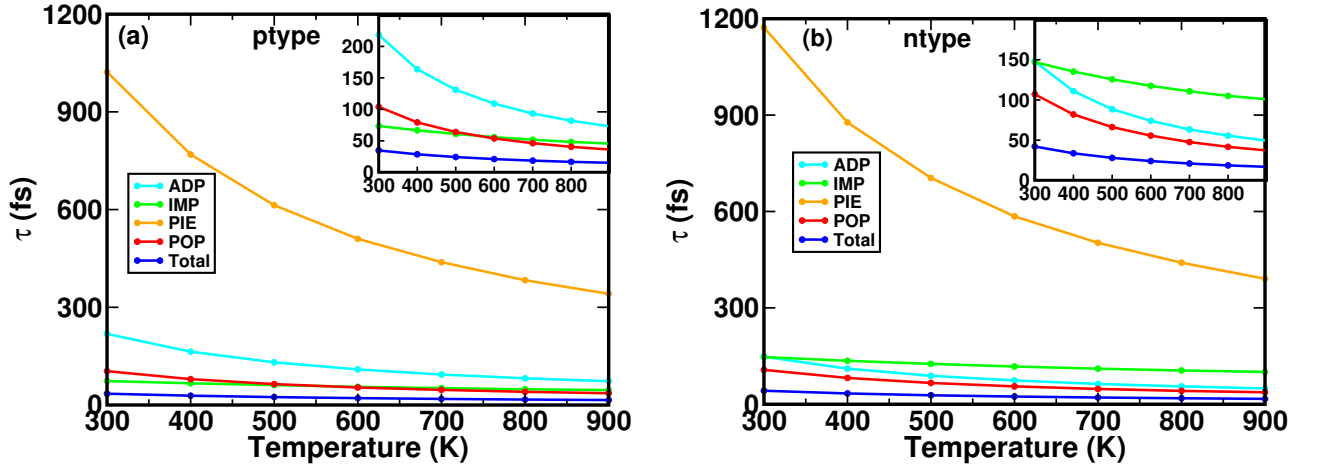

FIG. SII. Contribution of individual scattering rates at the optimised carrier concentration of  $4 \times 10^{19} \text{ cm}^{-3}$  for p-type and  $1 \times 10^{19} \text{ cm}^{-3}$  for n-type conduction for  $\text{Cu}_2\text{ZnSiTe}_4$ .

$$g_{nm}^{ii}(k, q) = \sum_{G \neq -q} \frac{n_{ii}^{1/2} Ze \langle mk + q | e^{i(q+G) \cdot r} | nk \rangle}{\hat{n} \cdot \epsilon_s \cdot \hat{n} |q + G|^2 + \beta^2} \quad (5)$$

where  $\beta$  is defined as

$$\beta = \frac{e^2}{\epsilon_s \kappa_B T} \int \frac{d\epsilon}{V} D(\epsilon) f(1 - f) \quad (6)$$

Figure SII shows the contribution of the individual scattering mechanisms at the optimized concentration of  $4 \times 10^{19} \text{ cm}^{-3}$  for p-type and  $1 \times 10^{19} \text{ cm}^{-3}$  for n-type in a temperature range of 300 to 900 K.

As it can be seen in figure SIV, Piezoelectric scattering is less dominant in comparison to other scatterings. PIE shows high relaxation time which means low scattering rates so it does not contribute significantly in transport mechanism. In the inset, we have shown the contribution from other scatterings, i.e., ADP, IMP and POP which are dominant scattering mechanisms in the 300-900 K temperature range.

- 
- [1] Alex M. Ganose, Junsoo Park, Alireza Faghaninia, Rachel Woods-Robinson, Kristin A. Persson, and Anubhav Jain. Efficient calculation of carrier scattering rates from first principles. *Nature Communications*, 12(1), April 2021.
